# Supplementary material for: On deceiving malware classification with section injection
Source: arXiv:2208.06092 source file (2022-08-12)
Supplement: Supplementary file 1 [file appendix.tex]

\appendix

%%%%%%%%%%%%%%%%

\section{}
